# Supplementary material for: Decomposing Chemical Space: Applications to the Machine Learning of Atomic Energies
Source: arXiv:2212.09489 ancillary file (2023-04-18)
Supplement: Supplementary file 1 [file si.pdf]

# Supporting Information: Decomposing Chemical Space: Applications to the Machine Learning of Atomic Energies

Frederik Ø. Kjeldal and Janus J. Eriksen*

*DTU Chemistry, Technical University of Denmark*

*Kemitorvet Bldg. 206, 2800 Kgs. Lyngby, Denmark*

E-mail: janus@kemi.dtu.dk

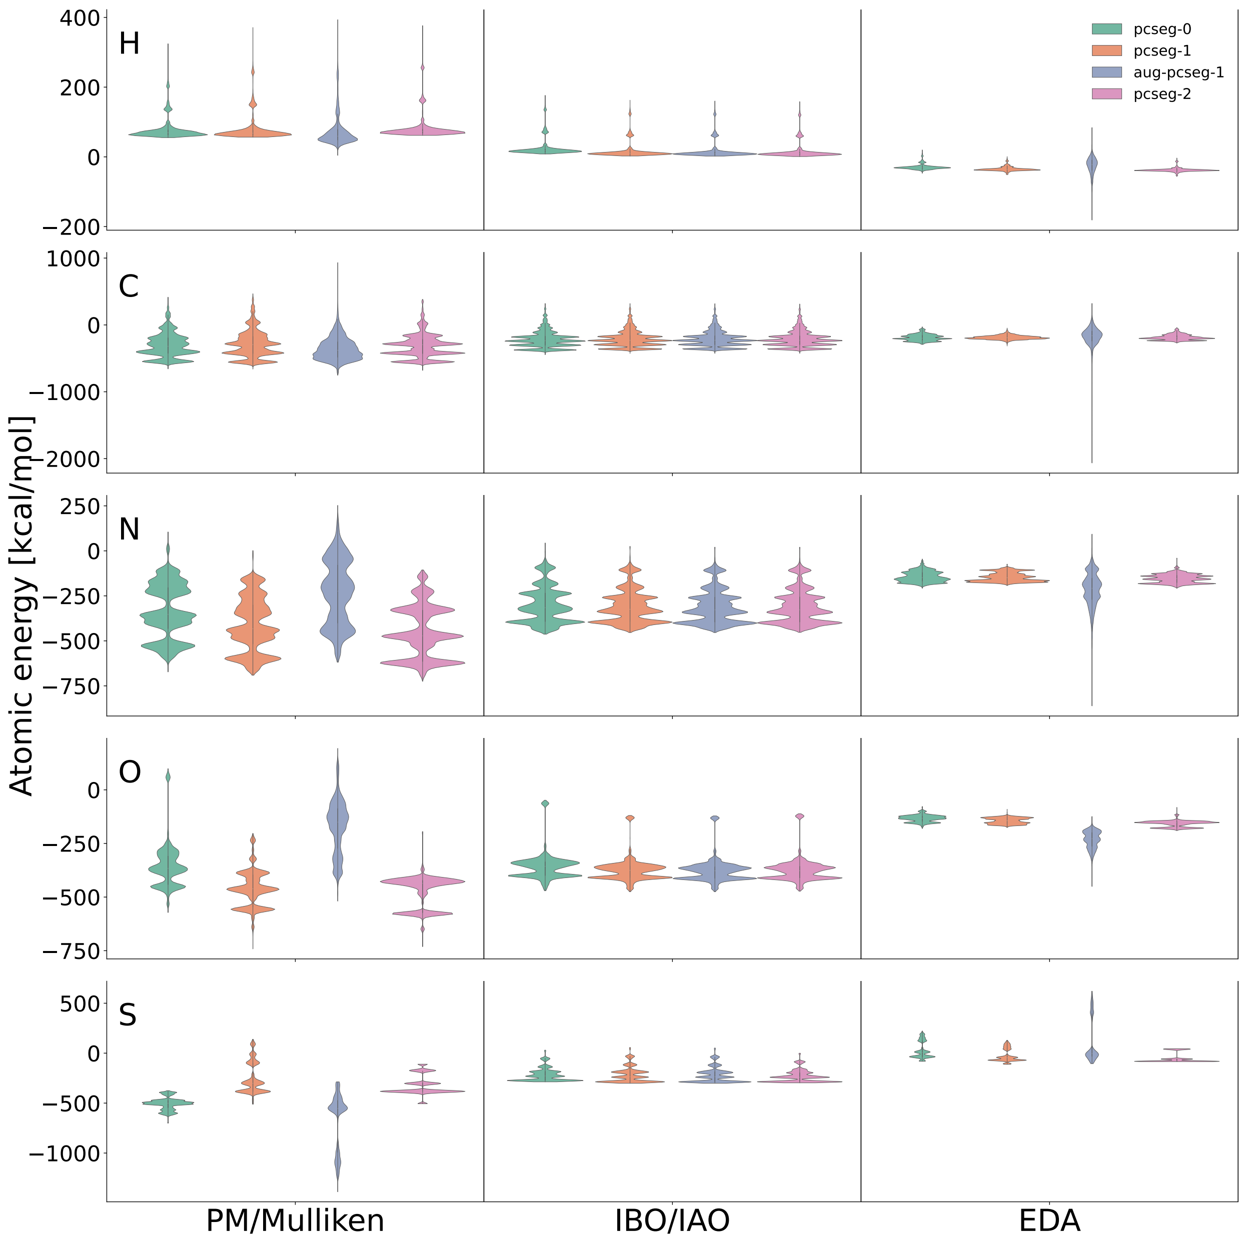


Figure S1: Atomization energies for all elements in the QM7 dataset using the B3LYP $xc$ functional and the (aug-)pcseg-$n$ basis sets ($n = 0, 1, 2$).

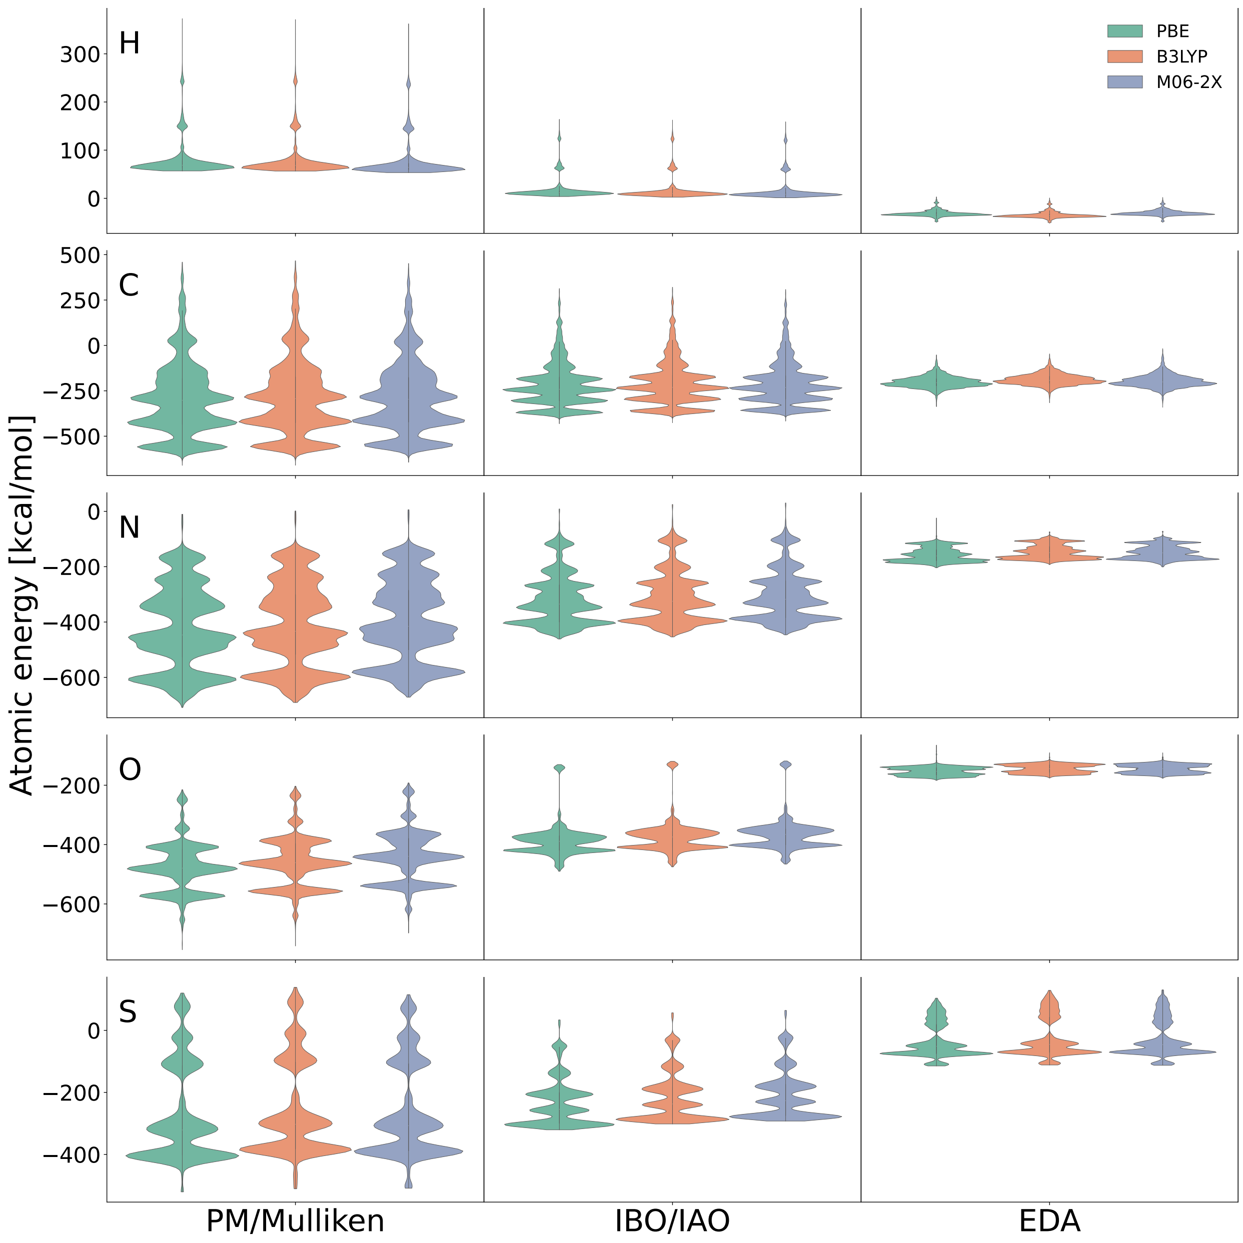


Figure S2: Atomization energies for all elements in the QM7 dataset using the PBE, B3LYP, and M06-2X *xc* functionals and the pcseg-1 basis set.

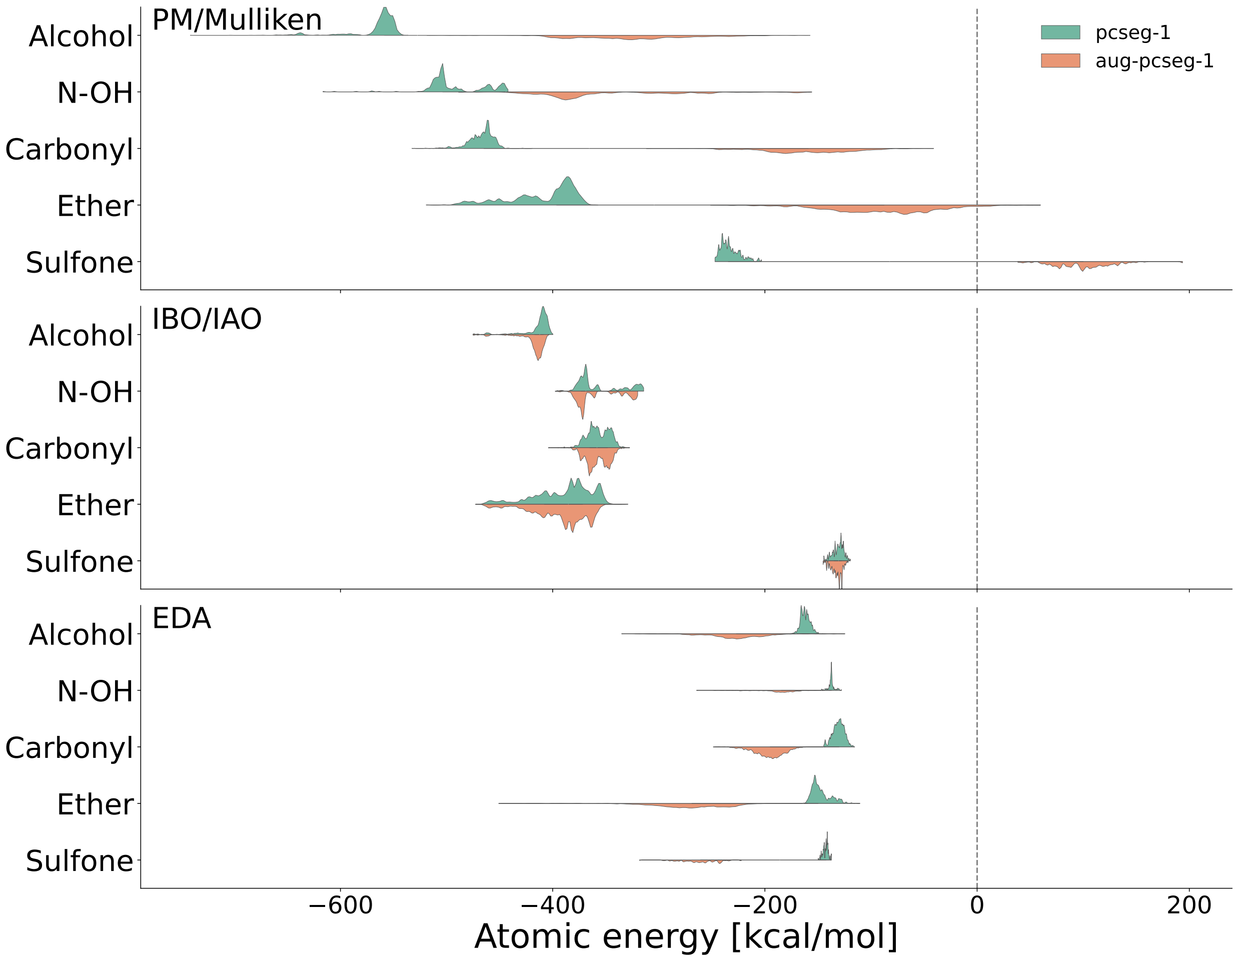


Figure S3: B3LYP/(aug-)pcseg-1 atomization energies for oxygen atoms of the most common functional groups in the QM7 dataset.

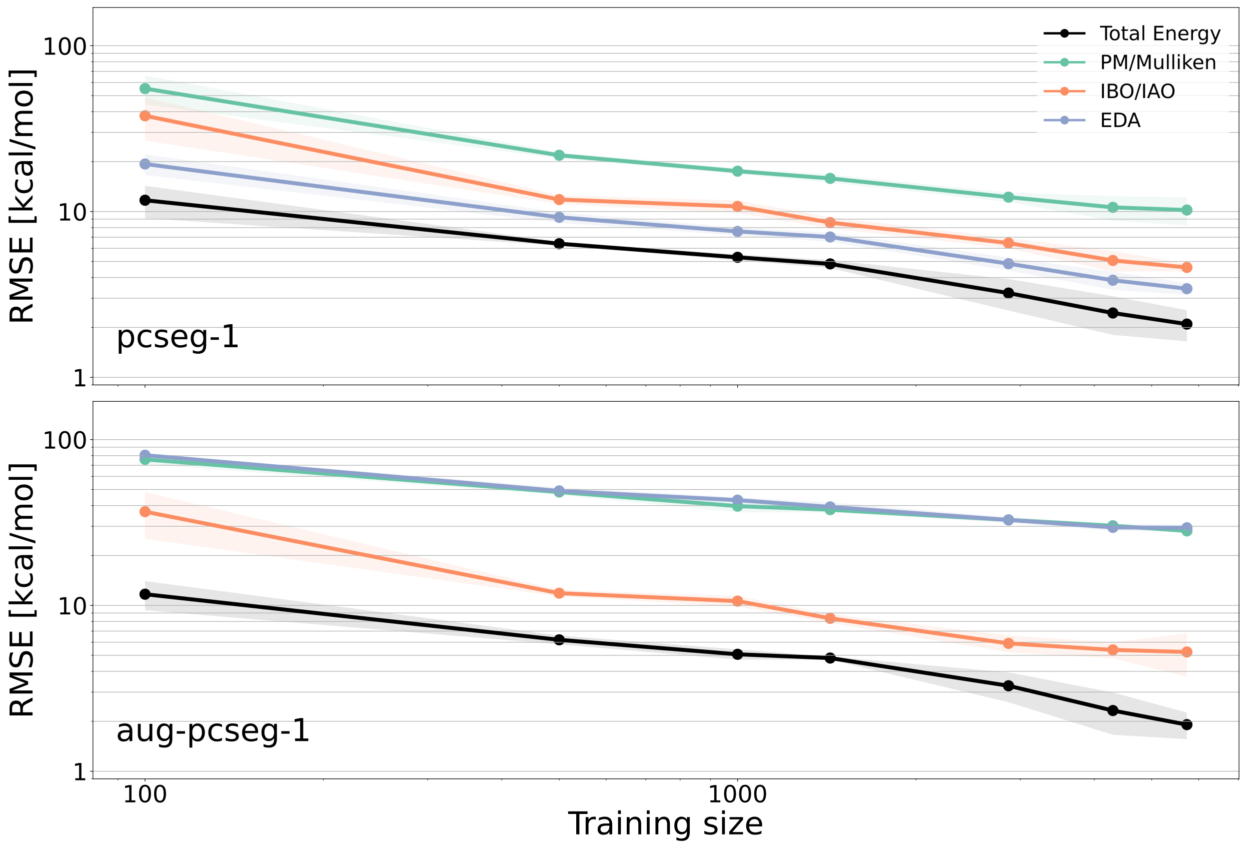


Figure S4: Same plot as Fig. 3 of the main study, but trained only on atomic energies.

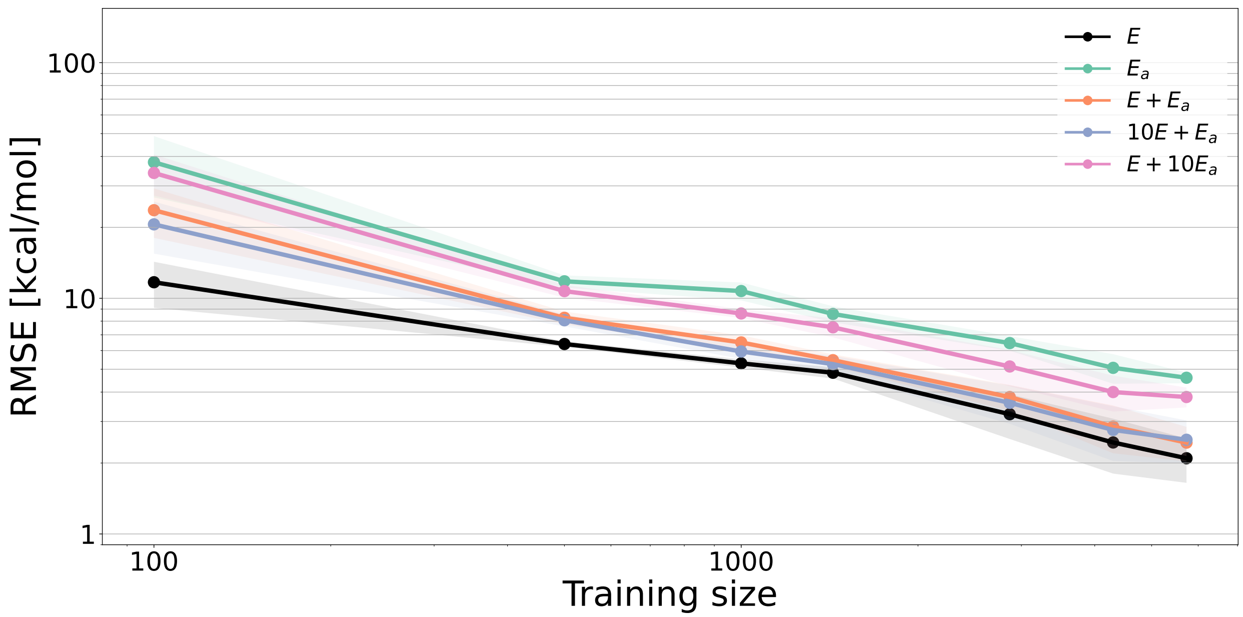


Figure S5: Total energy training curves (based on IBO/IAO data in the pcseg-1 basis set) obtained using different weightings of atomic ($E_a$) and molecular ($E$) energies.

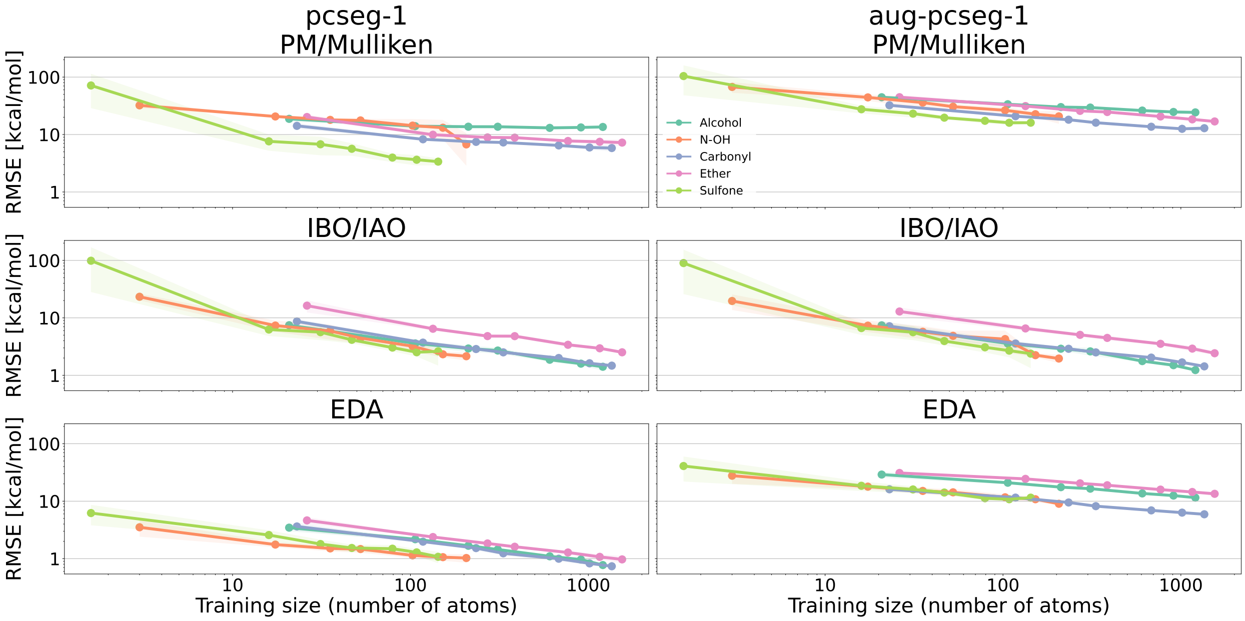


Figure S6: Training curves for the oxygen atoms in Fig. S3.

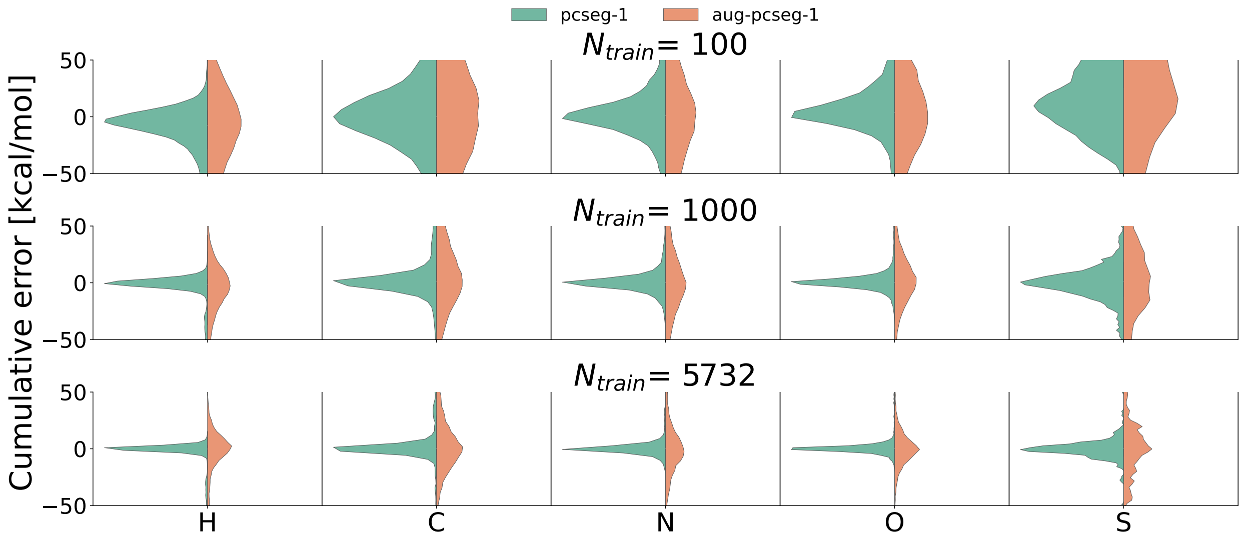


Figure S7: Same plot as Fig. 6 of the main study, but trained on PM/Mulliken data.

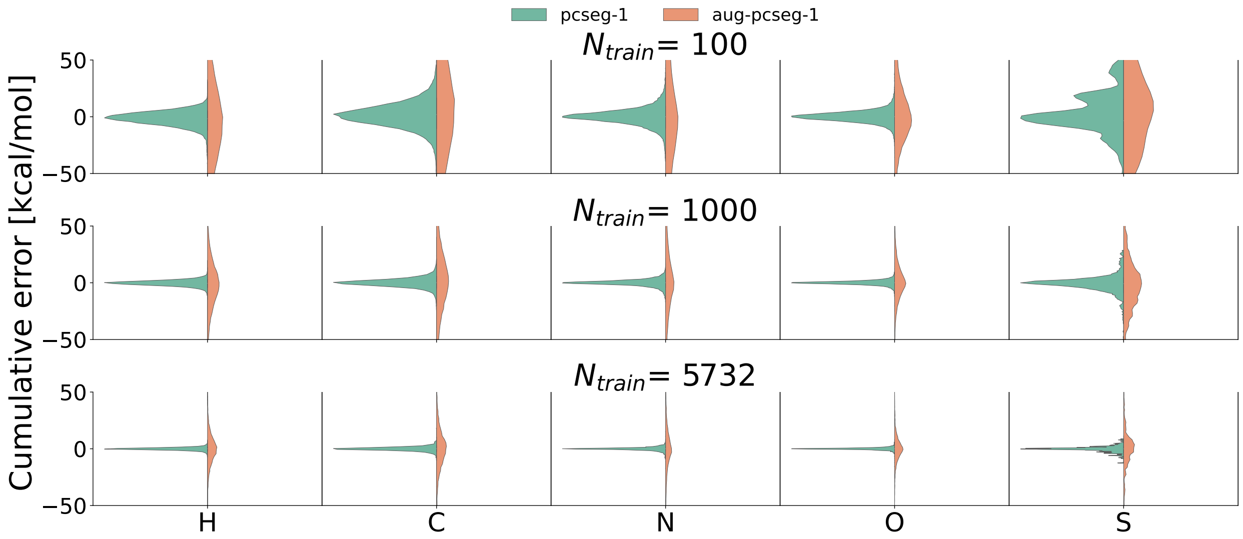


Figure S8: Same plot as Fig. 6 of the main study, but trained on EDA data.

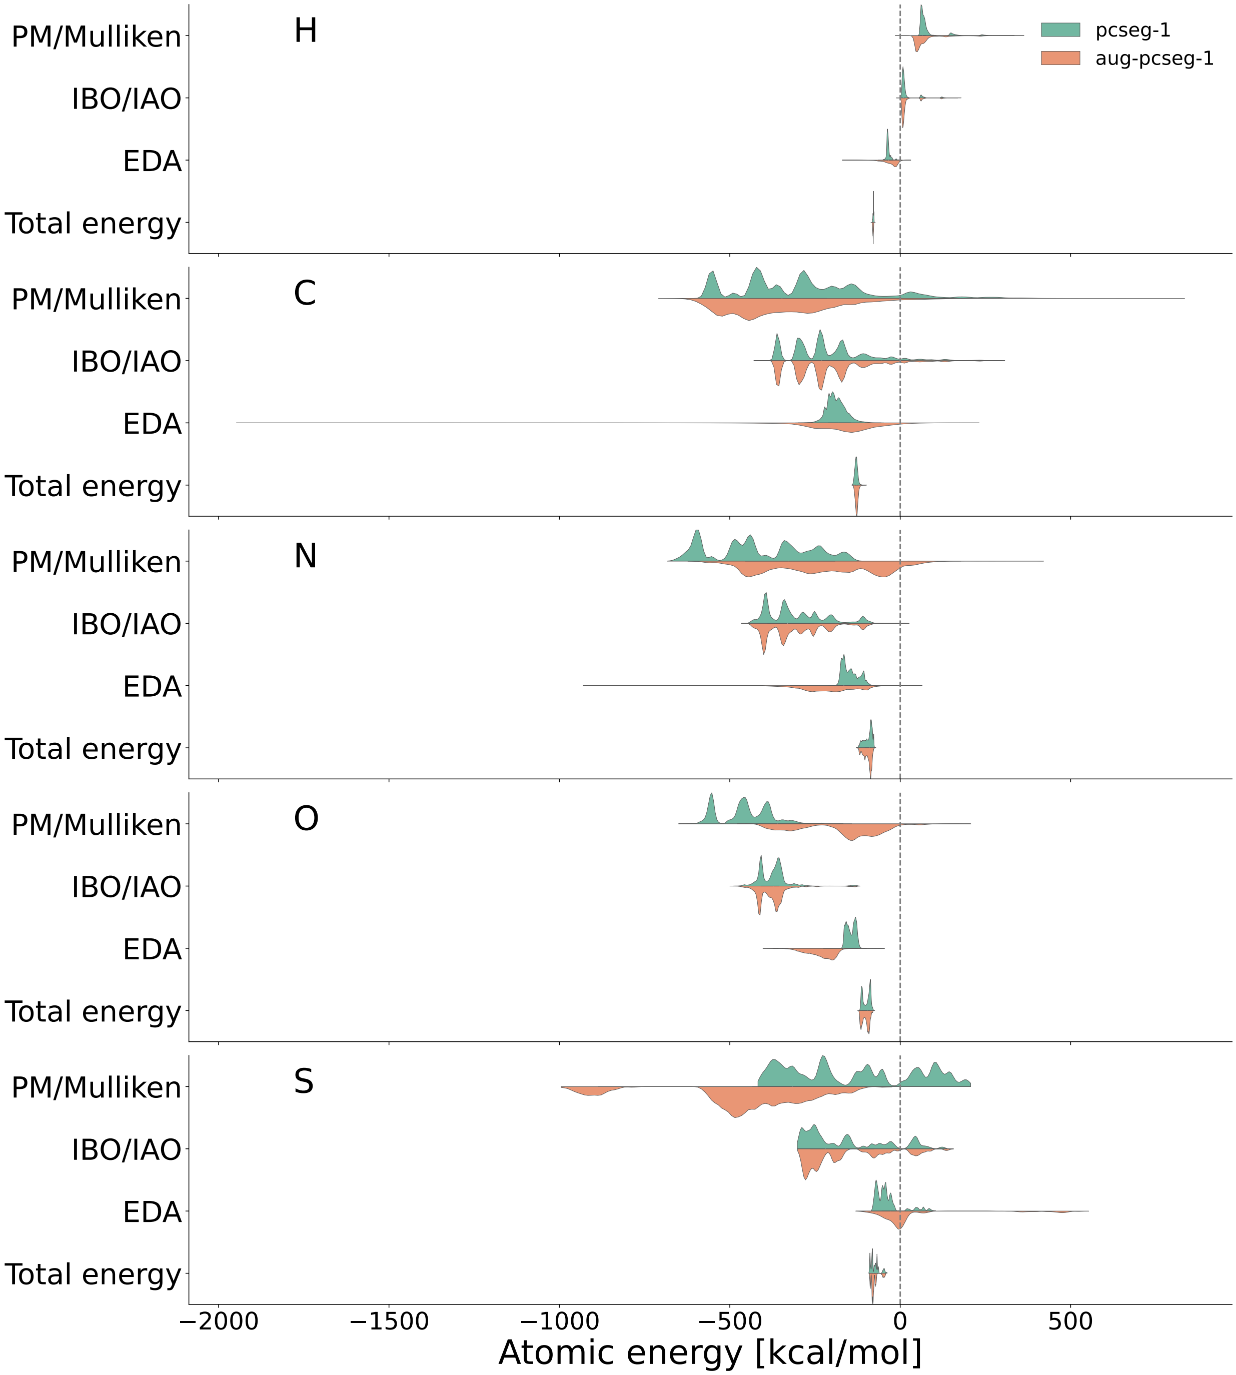


Figure S9: Predicted atomization energies from PhysNet NNs trained on an ensemble of 5 seeds with 100 random molecules each, using either total energies or data from any of the three atomic partitioning schemes as input.

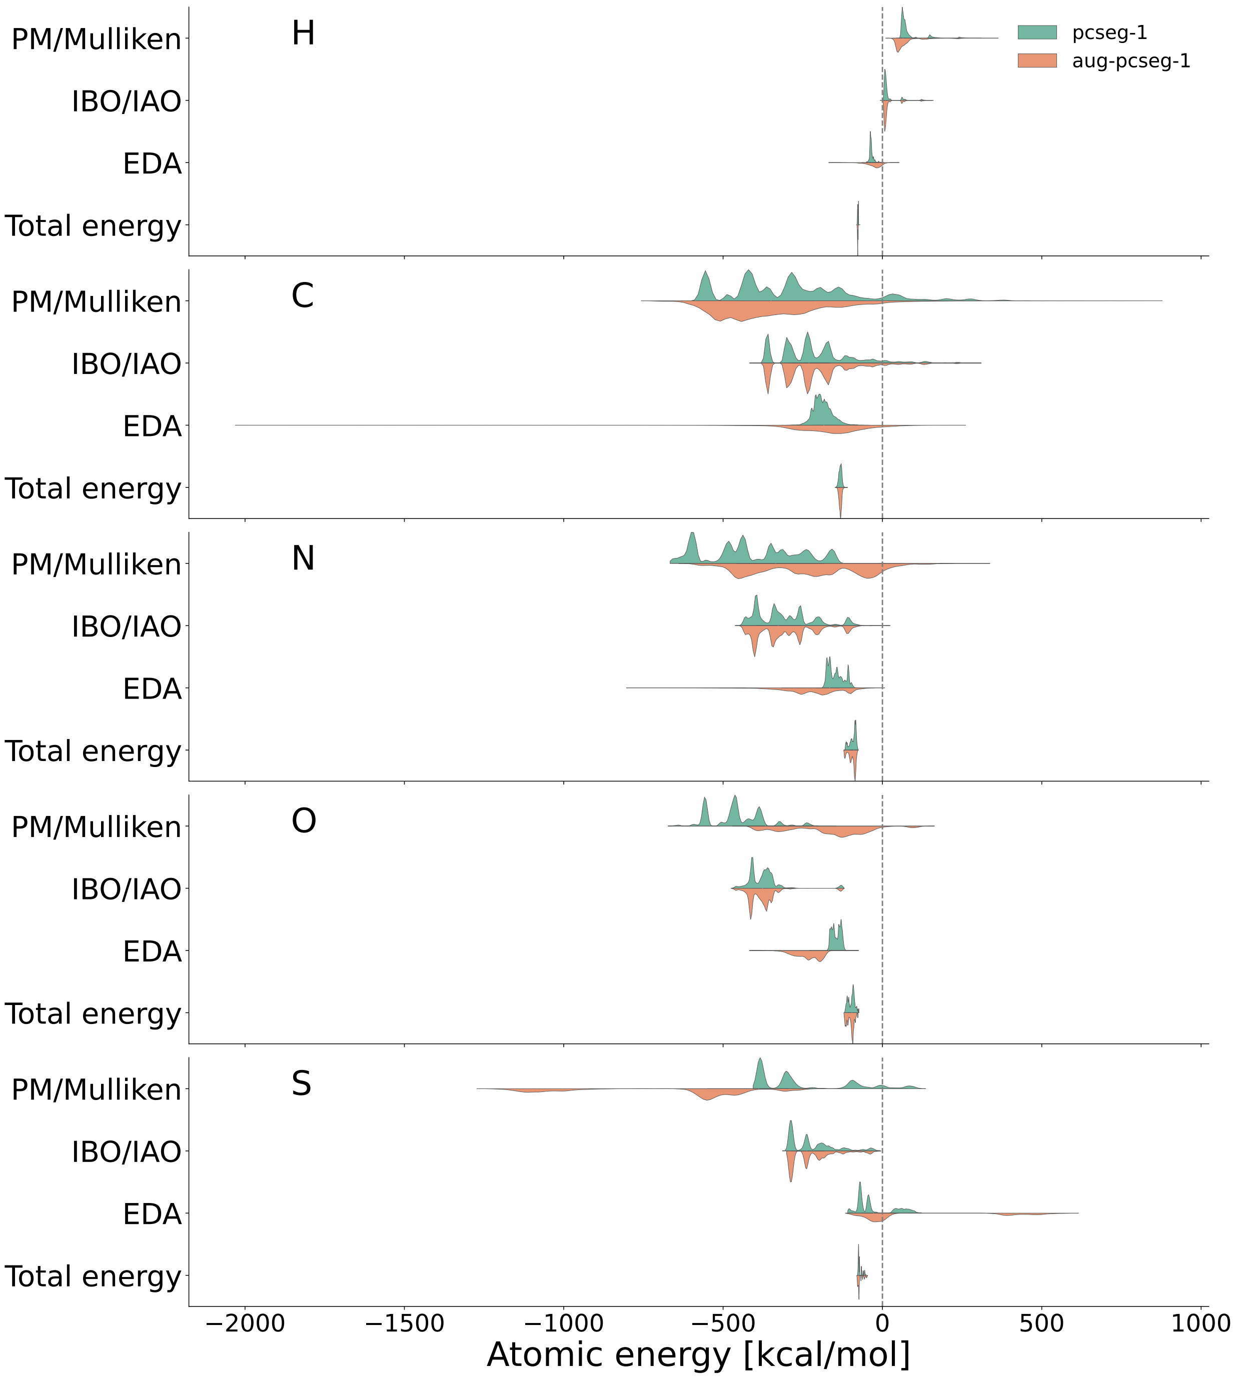


Figure S10: Same plot as Fig. S7, but trained on ensembles of 1000 molecules.

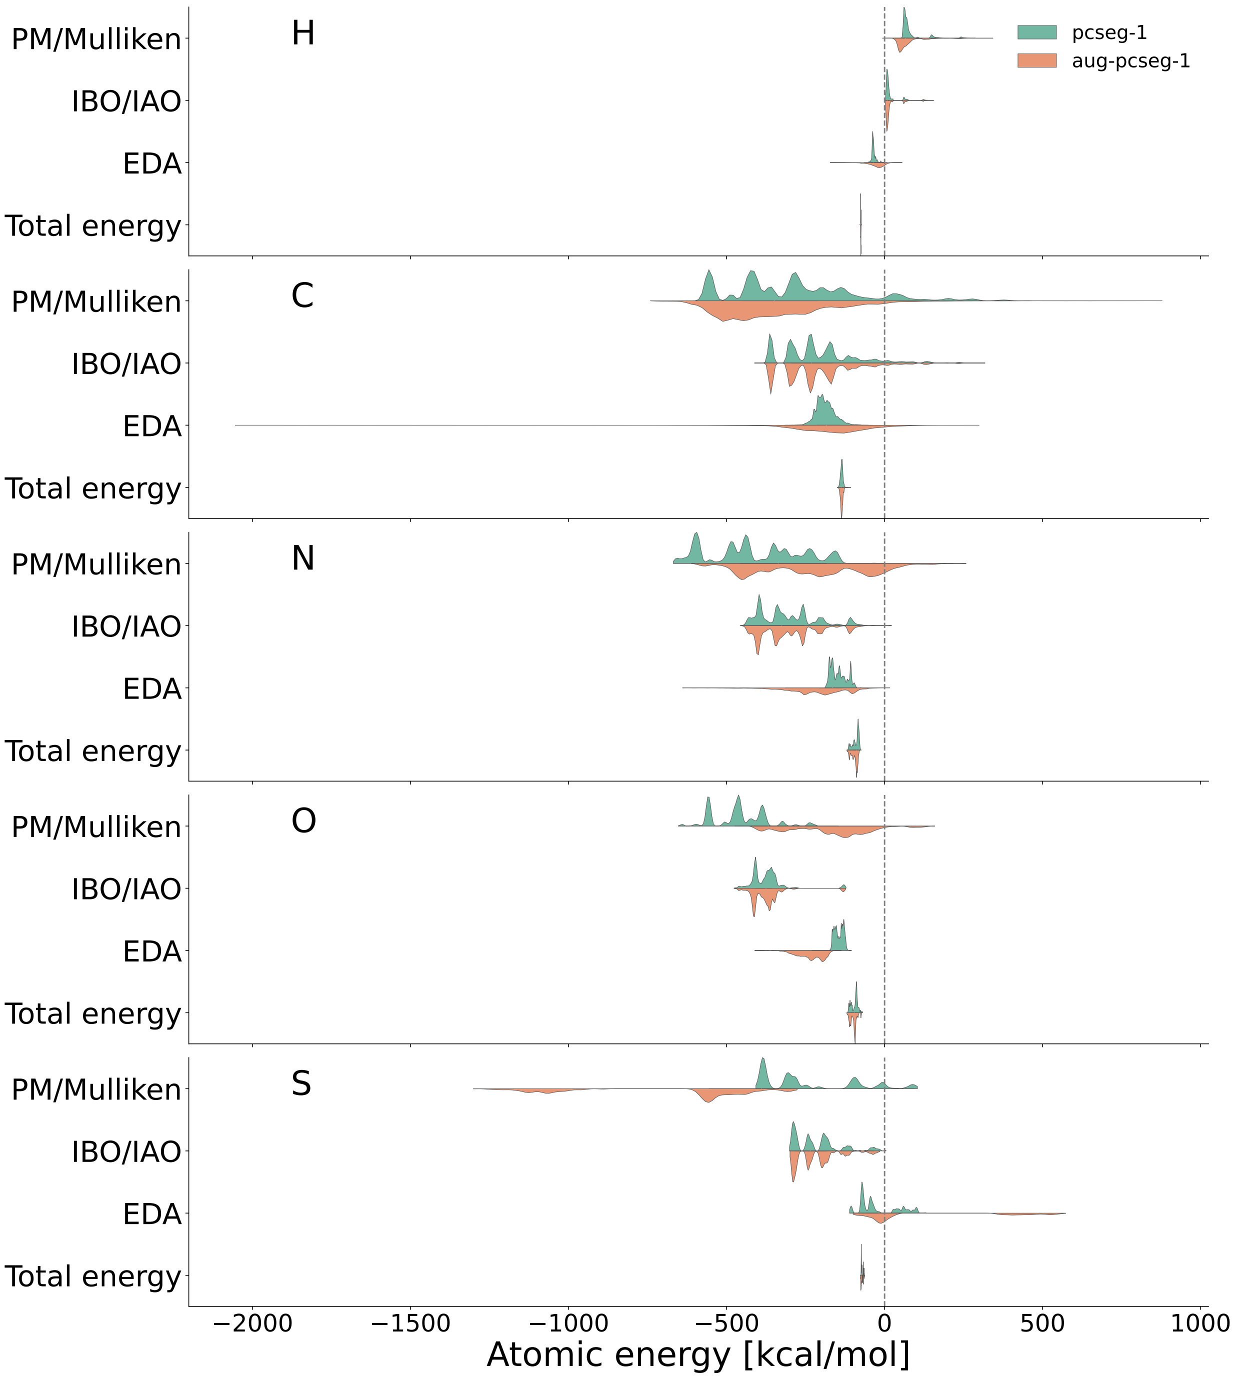


Figure S11: Same plot as Fig. S7, but trained on ensembles of 5732 molecules.

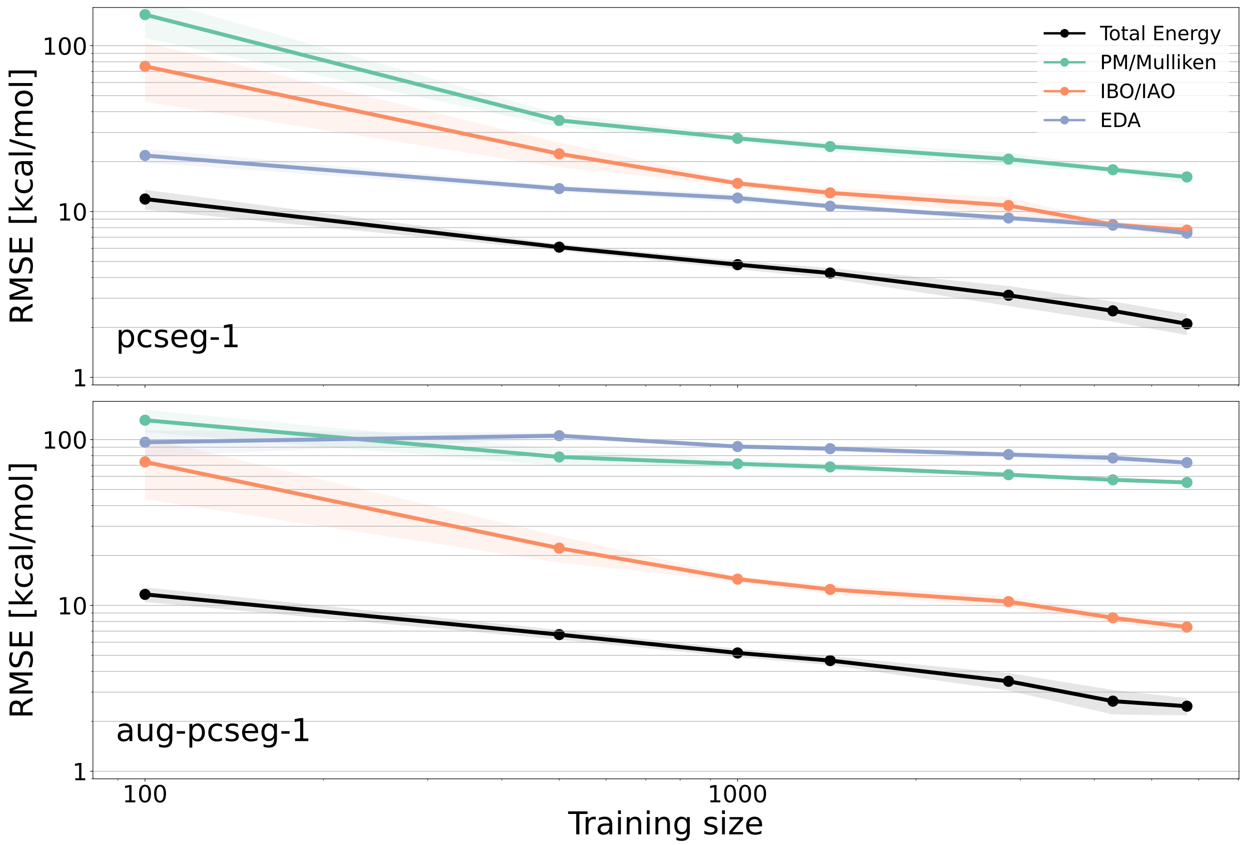


Figure S12: Same plot as Fig. 3 of the main study, but based on `ANI` NN architectures.

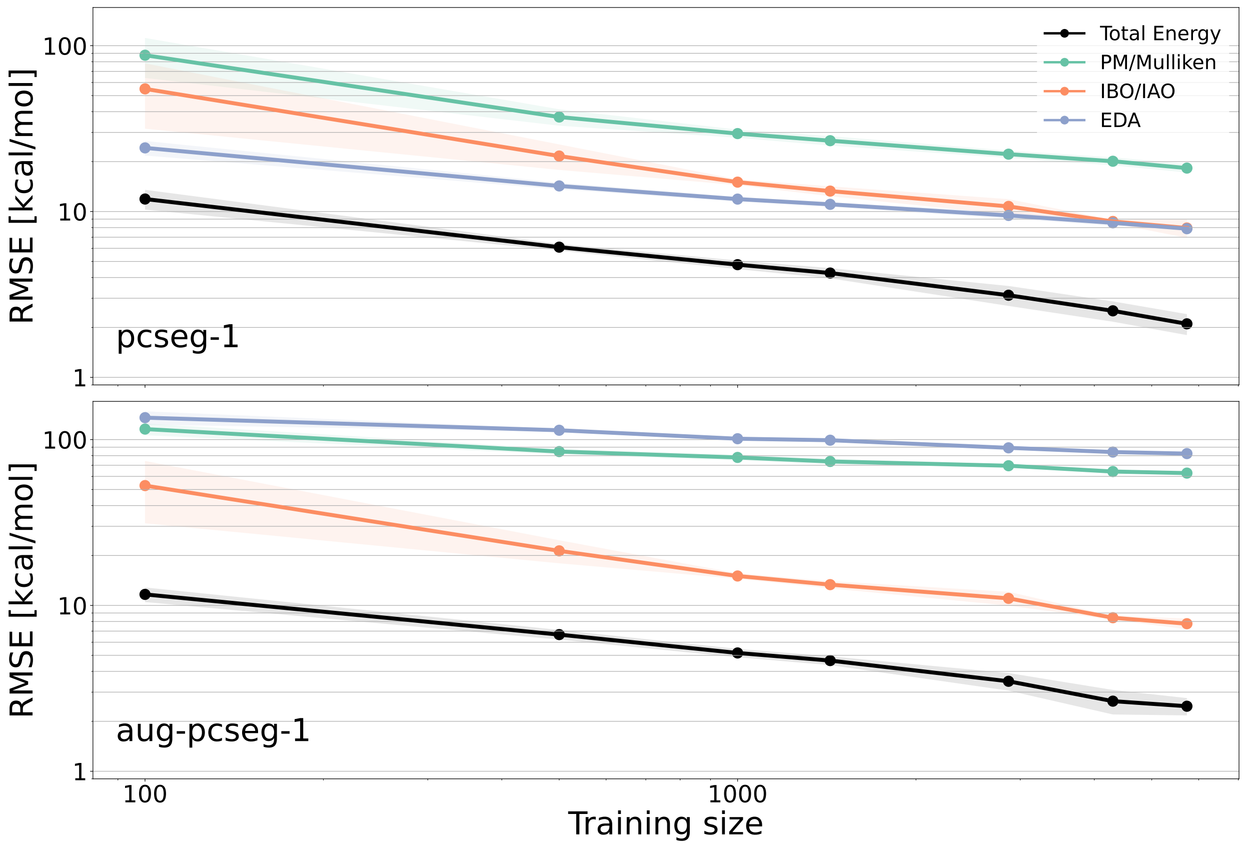


Figure S13: Same plot as Fig. S4, but based on `ANI` NN architectures.

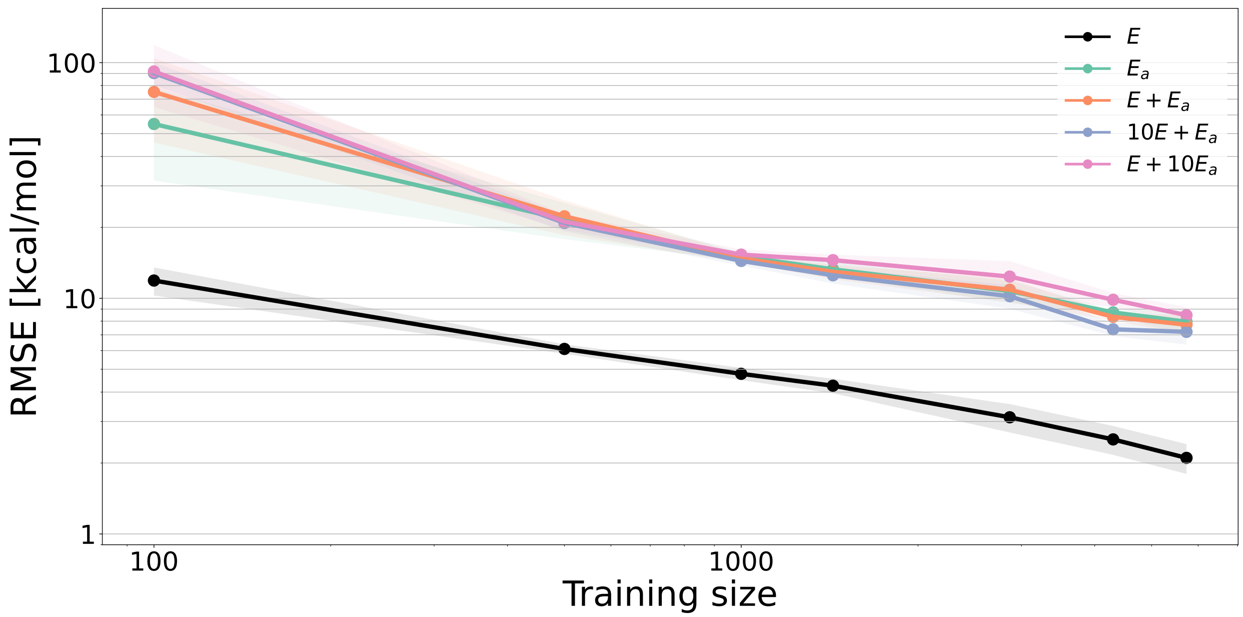


Figure S14: Same plot as Fig. S5, but based on ANI NN architectures.

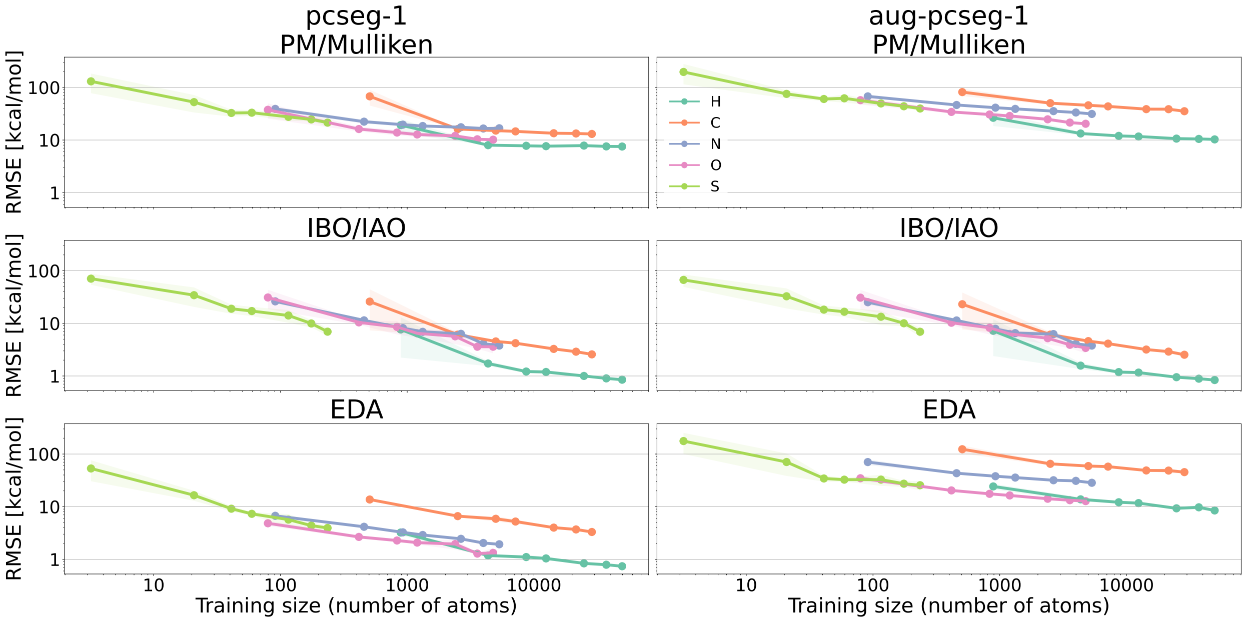


Figure S15: Same plot as Fig. 4 of the main study, but based on `ANI` NN architectures.

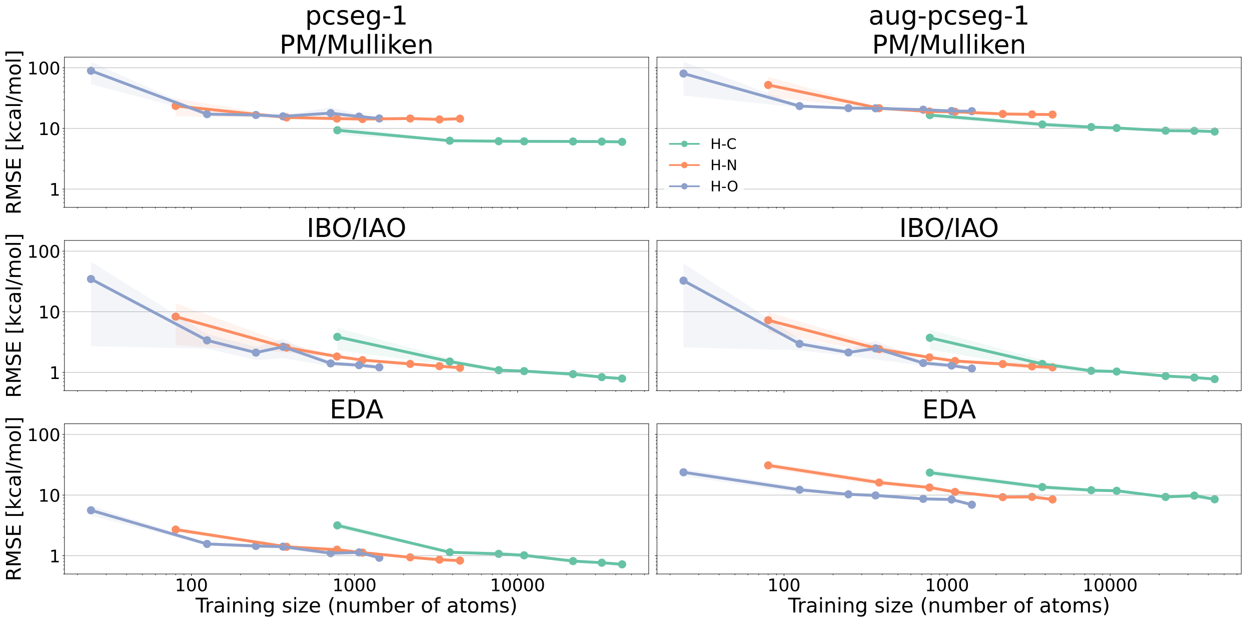


Figure S16: Same plot as Fig. 5 of the main study, but based on `ANI` NN architectures.

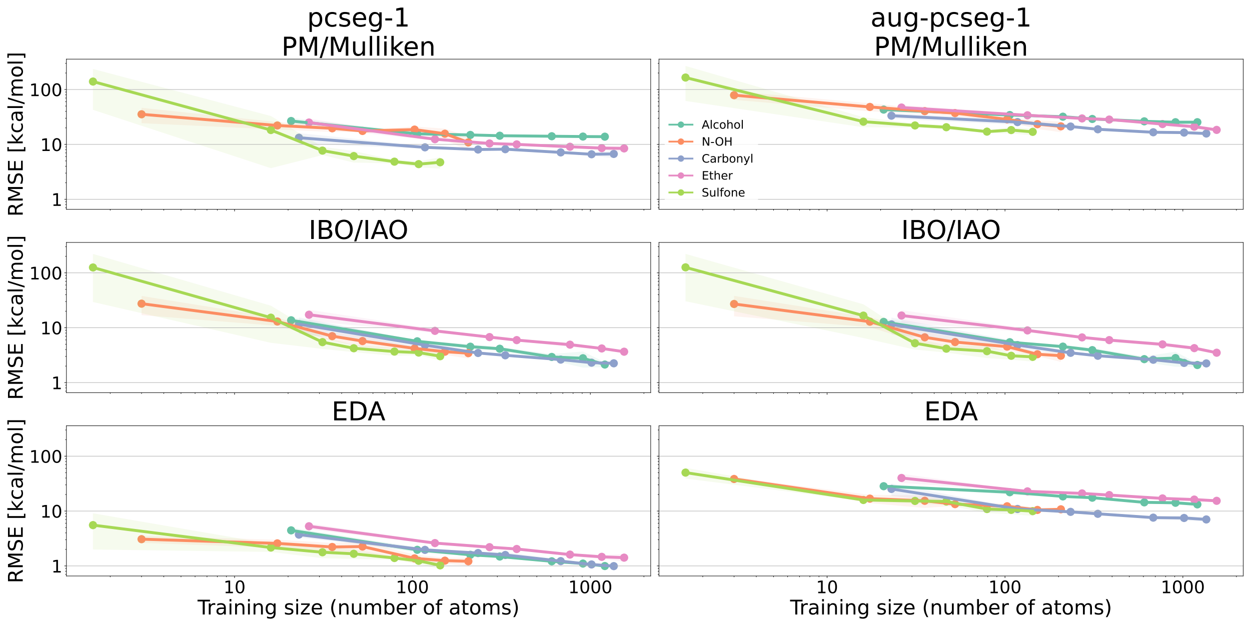


Figure S17: Same plot as Fig. S6, but based on `ANI` NN architectures.

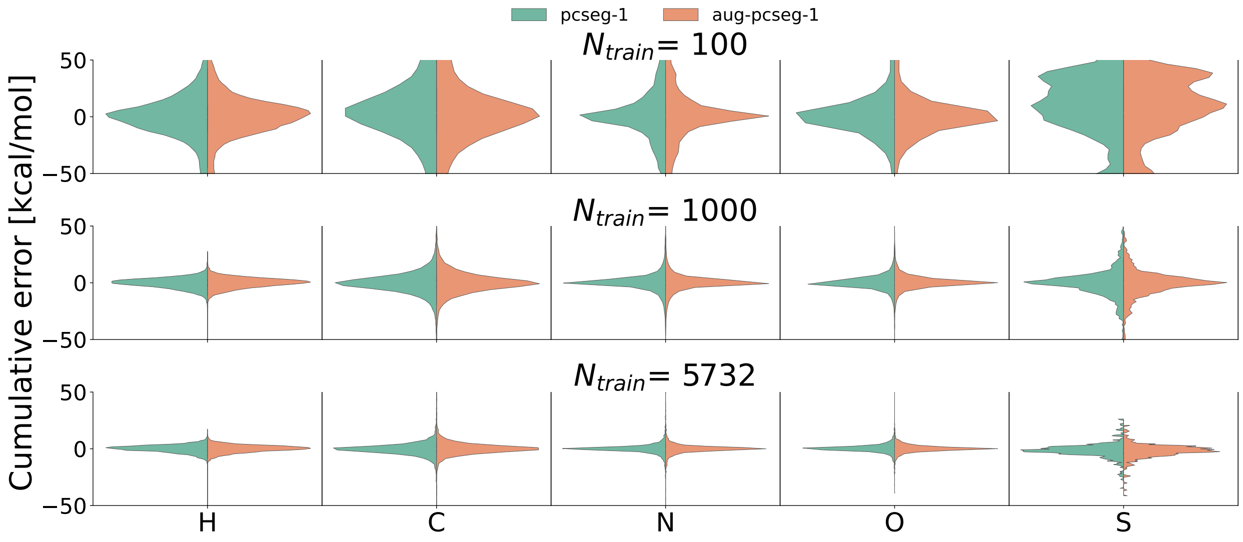


Figure S18: Same plot as Fig. 6 of the main study, but based on `ANI` NN architectures.

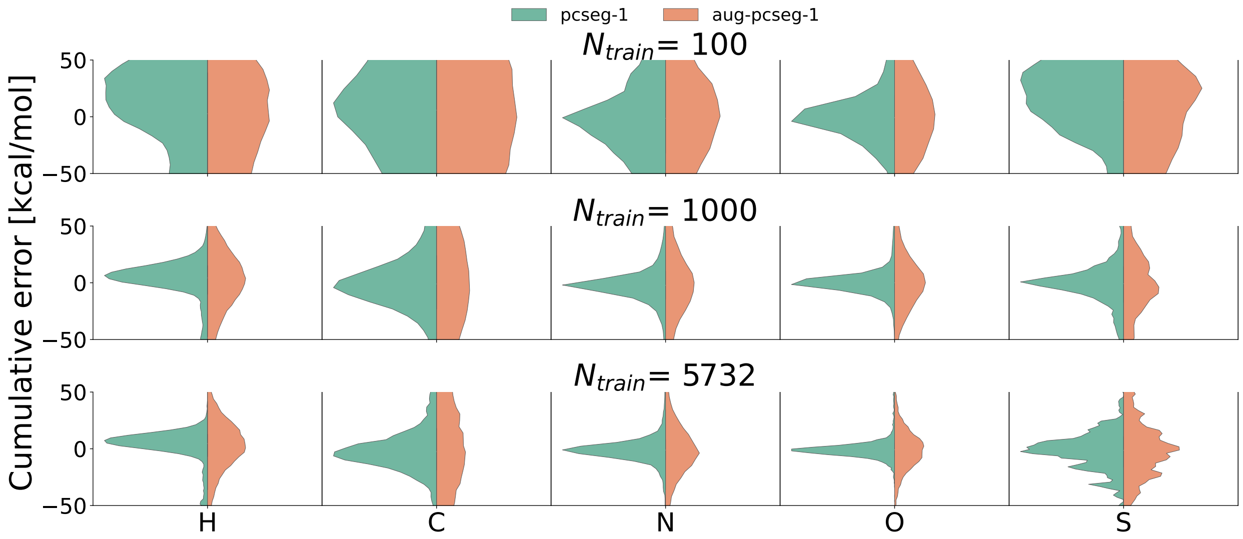


Figure S19: Same plot as Fig. S7, but based on `ANI` NN architectures.

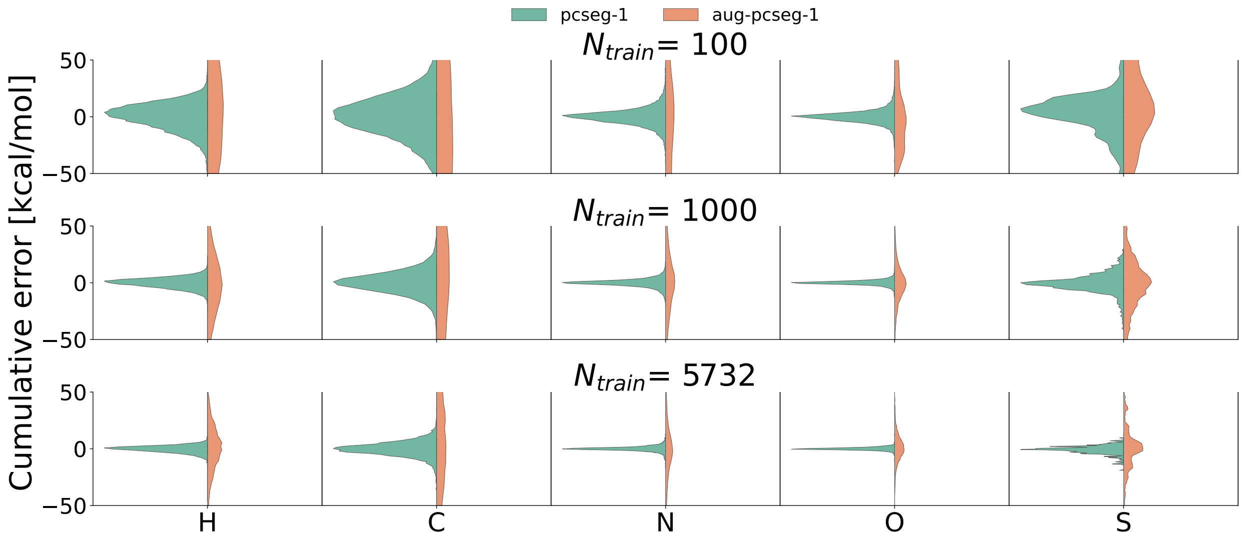


Figure S20: Same plot as Fig. S8, but based on `ANI` NN architectures.

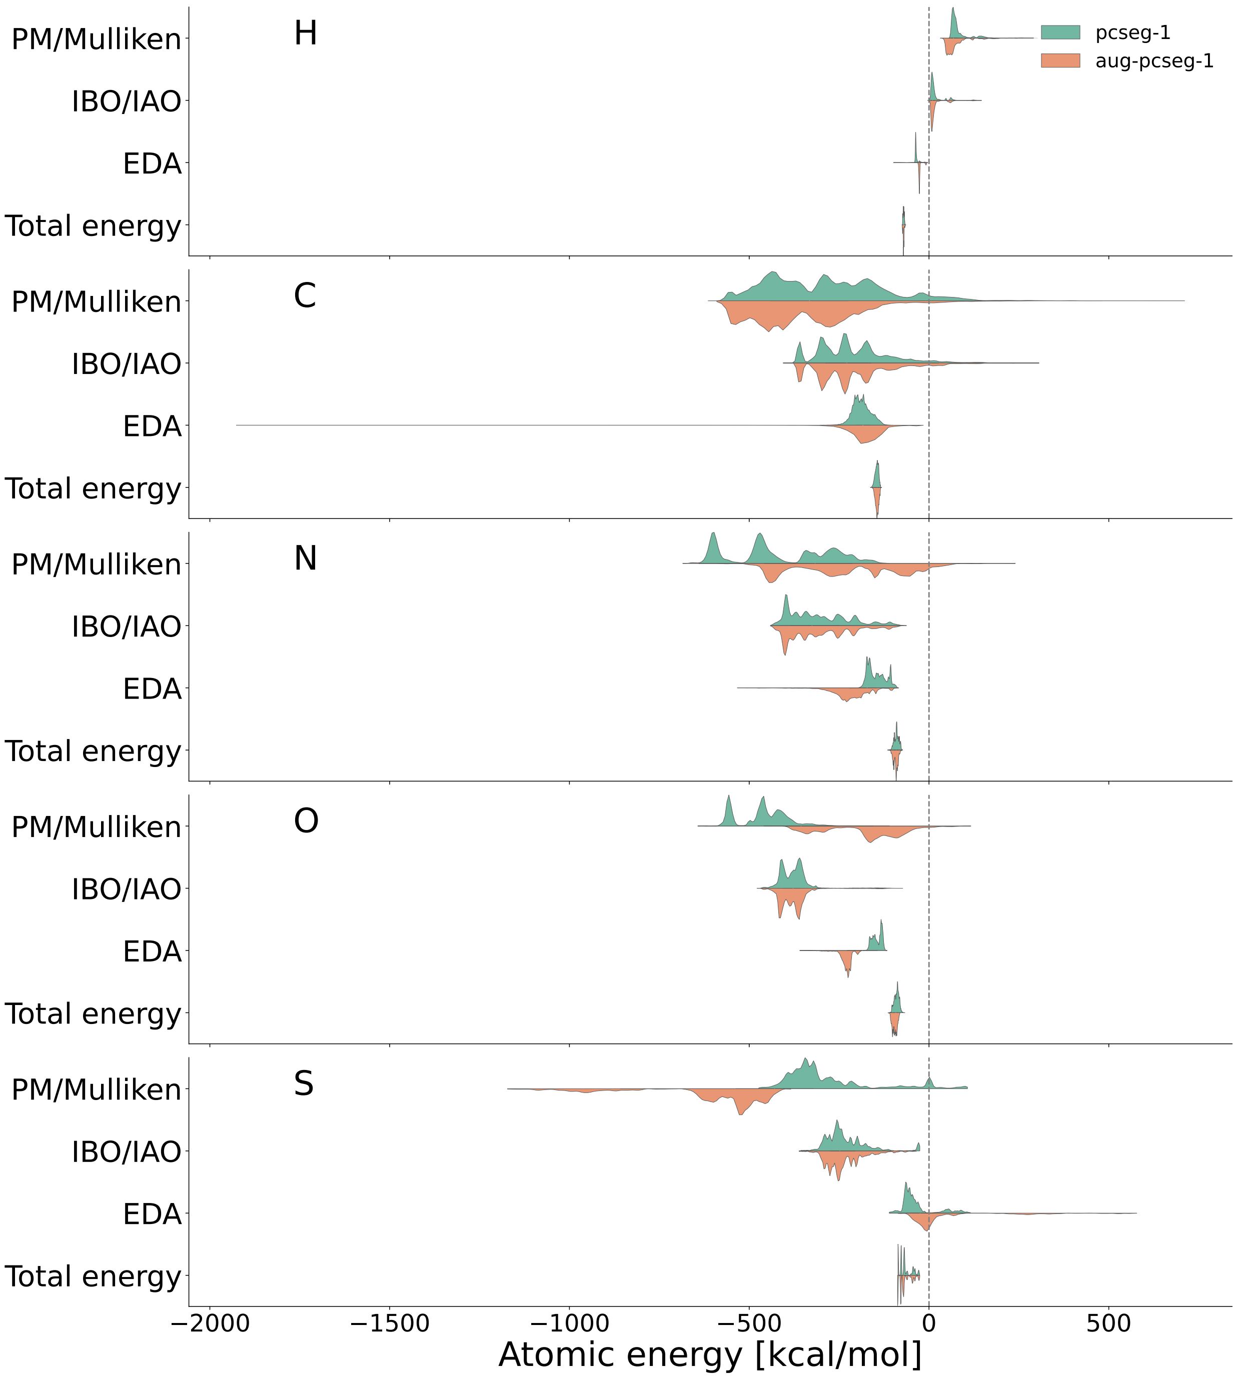


Figure S21: Same plot as Fig. S9, but based on `ANI` NN architectures.

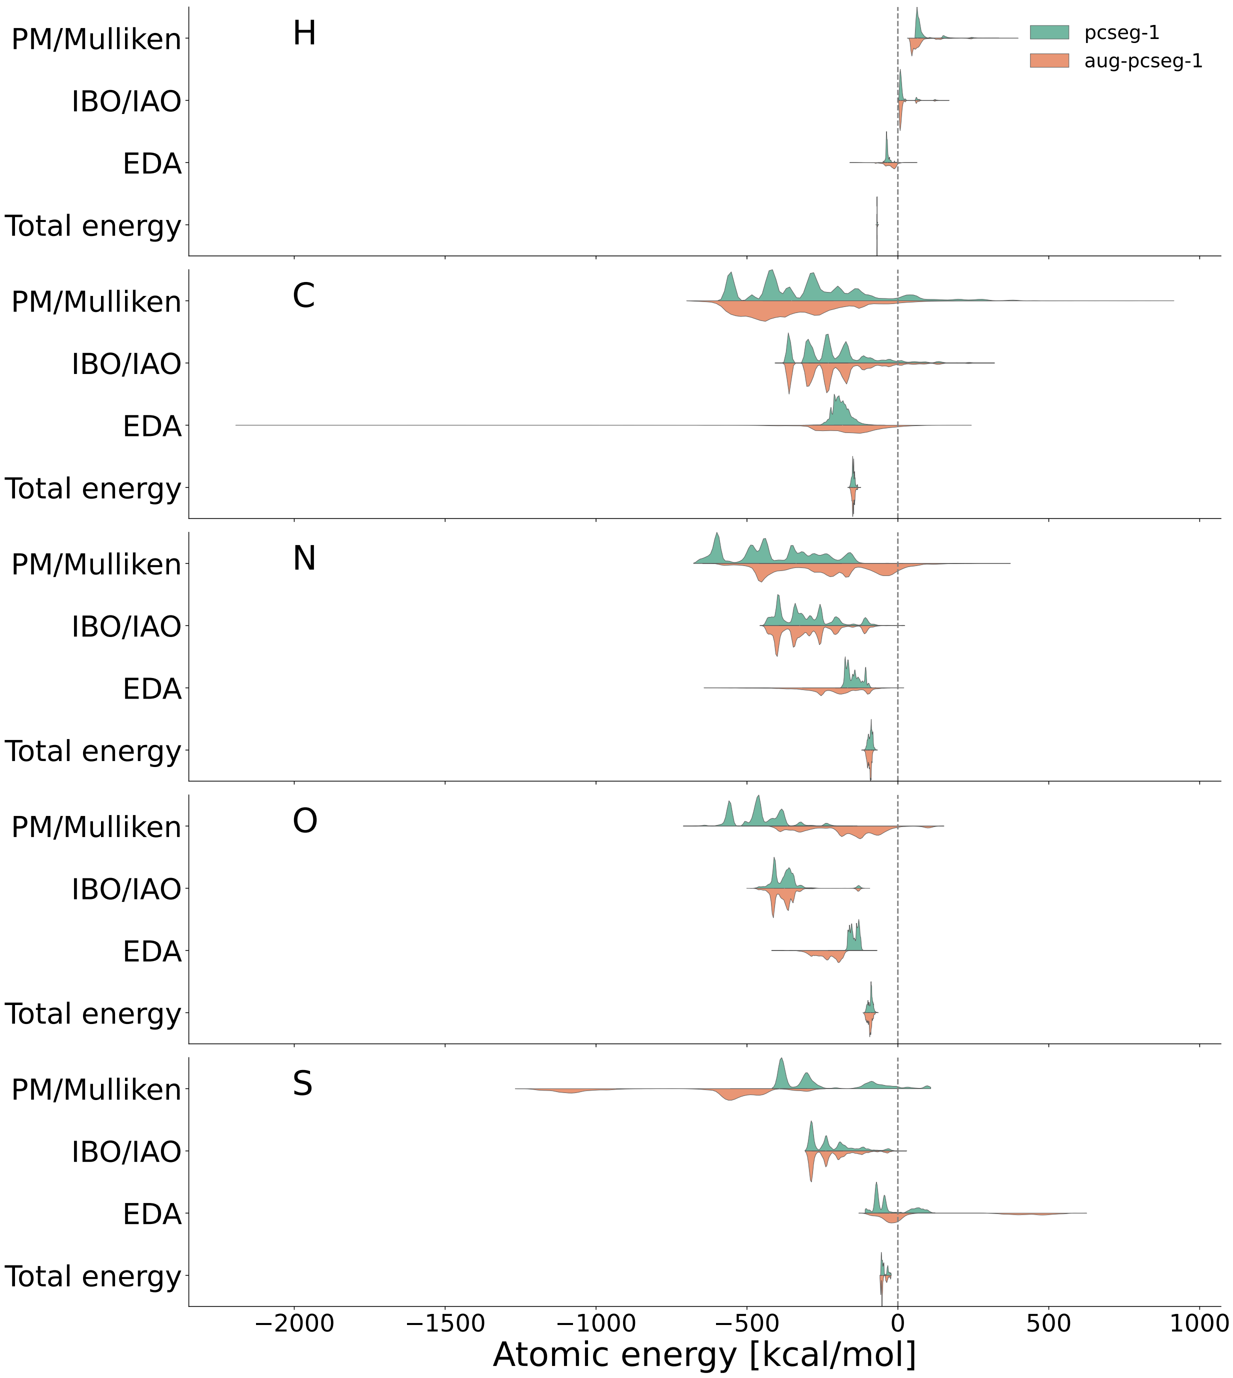


Figure S22: Same plot as Fig. S10, but based on ANI NN architectures.

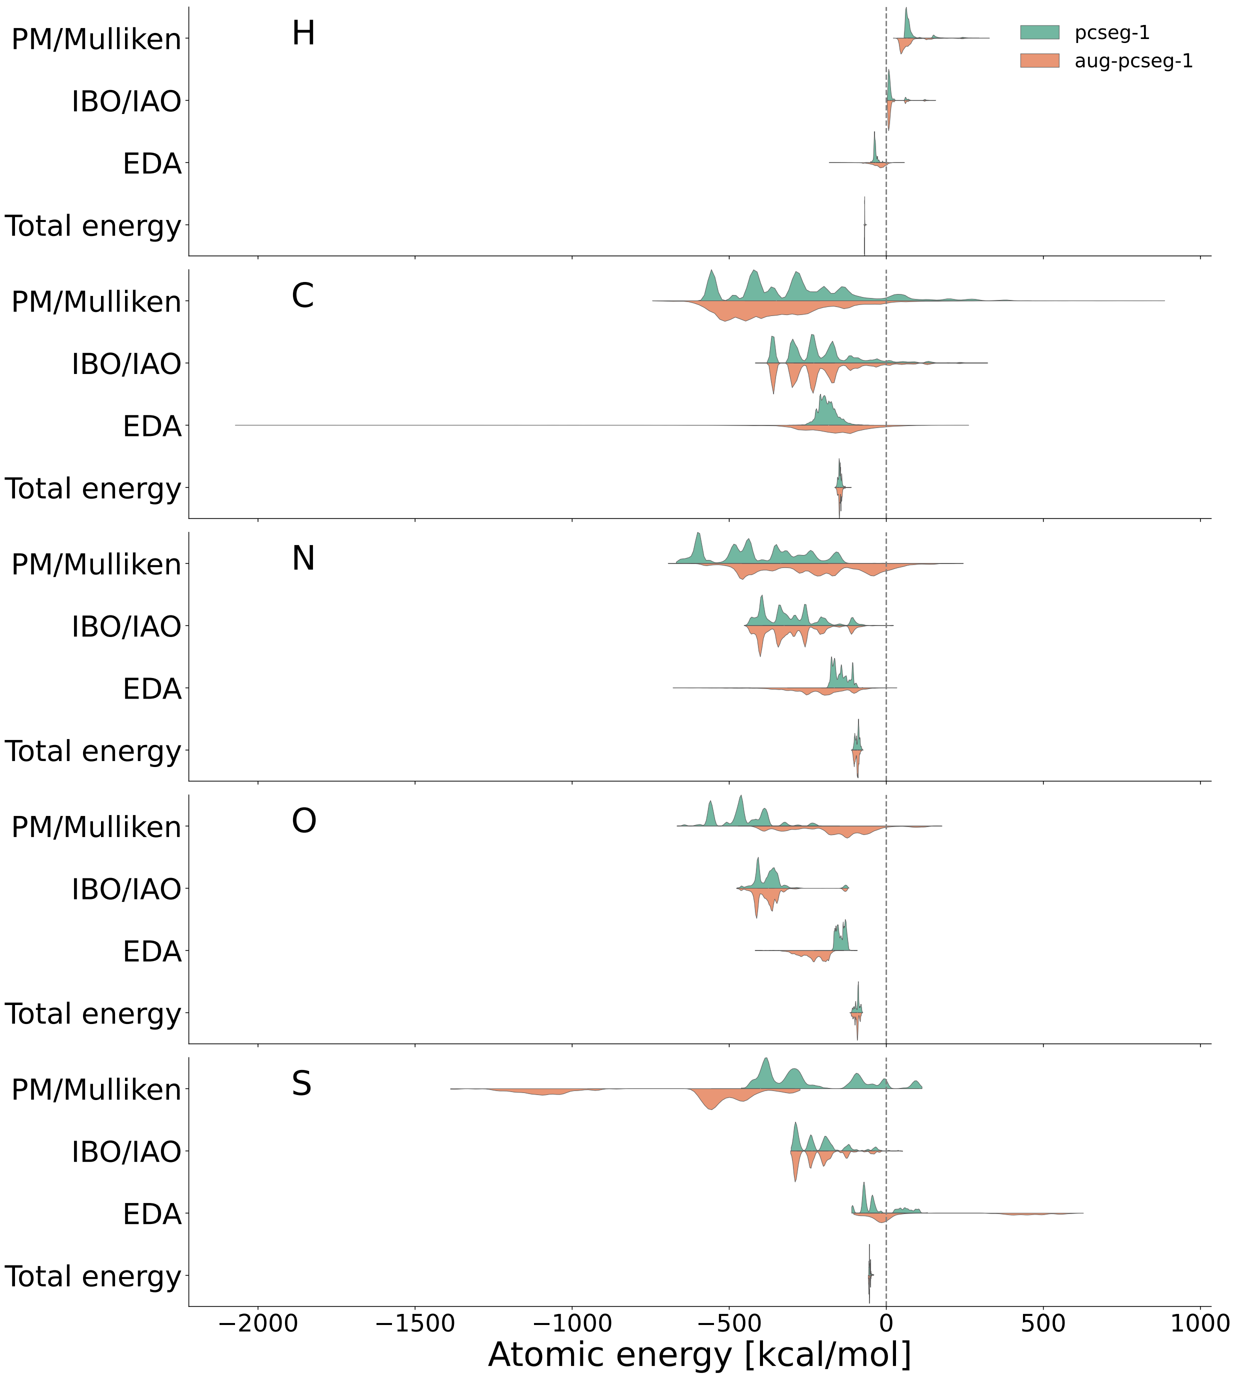


Figure S23: Same plot as Fig. S11, but based on `ANI` NN architectures.
